# Supplementary material for: WISE: Whitebox Image Stylization by Example-based Learning
Source: arXiv:2207.14606 source file (2022-07-29)
Supplement: Supplementary file 1 [file grid_template.tex]

\documentclass[runningheads]{llncs}
% DO NOT USE \usepackage{times}, it will be removed by typesetters
%\usepackage{times}

% INITIAL SUBMISSION - The following two lines are NOT commented
% CAMERA READY - Comment OUT the following two lines
% \usepackage{ruler}
% \usepackage[width=122mm,left=12mm,paperwidth=146mm,height=193mm,top=12mm,paperheight=217mm]{geometry}

% Include other packages here, before hyperref.
\usepackage{amsmath}
\usepackage{amssymb}
\DeclareMathOperator{\sign}{sign}
\usepackage[binary-units=true]{siunitx}
\DeclareSIUnit\pixel{P}
%https://tex.stackexchange.com/questions/403693/use-text-font-in-siunitx-instead-of-math-font
\sisetup{detect-all} 
\usepackage[super]{nth}

% % prevent Shipout twice included error
% \makeatletter
% \@namedef{ver@everyshi.sty}{}
% \makeatother

% \usepackage{comment}
% \usepackage[pdftex]{graphicx}
% \usepackage[labelformat=parens,labelsep=quad,skip=3pt]{caption}
% \usepackage[font=footnotesize]{subcaption}

%\usepackage[a4paper]{geometry}
% \usepackage{array}
% \usepackage{tikz}
% \usepackage{layouts}
% \usepackage{amsmath}
% \usepackage{amssymb}
 

\usepackage{csquotes}
\usepackage{subcaption}
\usepackage{color,soul}
\usepackage[edges]{forest}
\usepackage{blindtext}
\usepackage{wrapfig}
\usepackage{mwe}
\usepackage{nicefrac}
\usepackage{bm}
\usepackage{mathtools}
\usepackage{latexsym}
%\usepackage{commath}
\usepackage{tablefootnote}
\usepackage{adjustbox}
\usepackage{enumitem} 
\usepackage{pifont}
\usepackage{xfrac}
% tables
\usepackage{tabularx}
\usepackage{multirow}
\usepackage{array}
\usepackage{booktabs}
\usepackage{todonotes}
%\setlength{\heavyrulewidth}{1.5pt}
%\setlength{\abovetopsep}{4pt}
\usepackage{import}
\usepackage{placeins}
\usepackage{multido}


\usetikzlibrary{shadows.blur}
\usetikzlibrary{positioning}
\usetikzlibrary{arrows.meta}
\usetikzlibrary{positioning}
\usetikzlibrary{spy}


\begin{document}


\pagestyle{headings}
\mainmatter
\def\ECCVSubNumber{6063}  % Insert your submission number here
% INITIAL SUBMISSION 
%\begin{comment}

    % The paper headers
\markboth{Supplemental Material for ECCV Submission 6063}{Supplemental Material for ECCV Submission 6063}%


    \titlerunning{ECCV-22 submission ID \ECCVSubNumber} 
    \authorrunning{ECCV-22 submission ID \ECCVSubNumber} 
    \author{Anonymous ECCV submission}
    \institute{Paper ID \ECCVSubNumber}


\newcommand{\specFigSize}{0.235\textwidth}
\newcommand{\halfFigSize}{0.155\textwidth}
\newlength{\tempdima}
\newcommand{\rowname}[1]% #1 = text
{\rotatebox{90}{\makebox[\tempdima][c]{\text{#1}}}}
\setlength{\tabcolsep}{0.5mm} % separator between columns




##INPUT


\end{document}
